# Supplementary material for: Search for pair production of heavy vector-like quarks decaying into high-$p_T$ $W$ bosons and top quarks in the lepton-plus-jets final state in $pp$ collisions at $\sqrt{s}$=13 TeV with the ATLAS detector
Source: arXiv:1806.01762 source file (2018-06-05)
Supplement: Supplementary file 1 [file Appendix.tex]

\begin{figure}[htb!]
\centering
\includegraphics[width=0.8\textwidth]{figures/VLQSigBranching.pdf}
\caption{Relative fraction of events in both signal regions for the different decay modes of a vector-like $B$ pair with $m_B=1300$\,GeV and equal decay branching ratios of
\BR($B\rightarrow Wt$) = \BR($B\rightarrow Zb$) = \BR($B\rightarrow Hb$) = 1/3.}
\label{fig:SigAccept}
\end{figure}

\begin{figure}[h!]
\centering
\includegraphics[width=0.48\textwidth]{figures/Ljet3in_1.pdf}
\includegraphics[width=0.48\textwidth]{figures/BDTSR.pdf}
\caption{Pre-fit distributions for the hadronic $B$ quark candidate mass distributions ($m_B^{\mathrm{had}}$) (left) and the BDT output score in BDTSR (right). The lower panel shows the ratio of data to the expected background yields. The band represents the systematic uncertainty before the maximum-likelihood fit. Events in the overflow and underflow bins are included in the last and first bin of the histograms, respectively. The expected $B\bar{B}$ signal corresponding to $m_{B} = 1300$ \GeV{} for a branching ratio of 100\% into $WtWt$ is also shown overlaid.}
\label{fig:PreFit}
\end{figure}

\begin{figure}[h!]
\centering
\includegraphics[width=0.8\textwidth]{figures/Ranking.pdf}
\caption{Ranking of nuisance parameters based on the fit to data in the signal-plus background hypothesis according to their effect on the uncertainty in $\mu$ ($\Delta \mu$). The $B\bar{B}$ signal hypothesis corresponds to $m_B = 1300$ \GeV{} for a branching ratio of 100\% into $WtWt$.
The open boxes show the initial impact of that source of uncertainty in the precision of $\mu$.
The filled blue area shows the impact on the measurement of that source of uncertainty, after the profile likelihood fit at the $+1\sigma$ level. The filled cyan region illustrates the same for the $-1\sigma$ impact (postfit). Both of those types of areas refer to the top axis.
The ranking from top to bottom is done according to the effect on $\mu$ after the fit.
The black points and associated error bars show the fitted value of the nuisance parameters and their errors and refer to the bottom axis; a mean of zero and a width of one would imply no constraint due to the profile likelihood fit.
Only the 20 highest ranked uncertainties are shown.
No nuisance parameter pull is shown for the statistical uncertainty, the Monte Carlo (MC) statistical component per bin, and the unconstrained \ttbar{} normalisation ($\mu_{\ttbar{}}$) parameter.
}
\label{Fig:Ranking}
\end{figure}

\begin{figure}[htb!]
\centering
\subfloat[]{\includegraphics[width=0.8\textwidth]{figures/signalAcceptance_WtWt.pdf}}\\
\subfloat[]{\includegraphics[width=0.8\textwidth]{figures/signalAcceptance_singlet}}
\caption{The signal efficiency times acceptance as a function of VLQ mass assuming 100~$\%$
  decay into $Wt$ (a) and the SU(2) singlet (b) for the two signal regions.}
\label{fig:sub:SigAccept}
\end{figure}

\begin{figure}[htb!]
\centering
\subfloat[]{\includegraphics[width=0.8\textwidth]{figures/SRs_hadB_m_singlet.pdf}}\\
\subfloat[]{\includegraphics[width=0.8\textwidth]{figures/bdtIn_BDToutX_allVars20_singlet.pdf}}
\caption{The reconstructed hadronic B quark mass in the RECOSR (top) and the BDT discriminant in BDTSR (bottom) is shown for the total expected background and a few signal mass points for the SU(2) singlet case. In both figures, the distributions are normalised to unity for comparison of the relative shapes at each mass point.}
\label{fig:disc_singlet}
\end{figure}

\begin{figure}[h!]
\centering
\includegraphics[width=0.44\textwidth]{figures/bdtIn_ST.pdf}
\includegraphics[width=0.44\textwidth]{figures/bdtIn_hadleadLjet_m.pdf}

\includegraphics[width=0.44\textwidth]{figures/bdtIn_spericity.pdf}
\includegraphics[width=0.44\textwidth]{figures/bdtIn_dR_lepsleadjet.pdf}

\includegraphics[width=0.44\textwidth]{figures/bdtIn_dR_leadbjetleadLjet.pdf}
\includegraphics[width=0.44\textwidth]{figures/bdtIn_mindR_lepbjet.pdf}

\includegraphics[width=0.44\textwidth]{figures/bdtIn_aplanarity.pdf}
\includegraphics[width=0.44\textwidth]{figures/bdtIn_Wlepb_minmass.pdf}

\includegraphics[width=0.44\textwidth]{figures/bdtIn_dR_lepthirdleadjet.pdf}
\includegraphics[width=0.44\textwidth]{figures/bdtIn_dR_WlepLjetCloseToBlead.pdf}

\caption{ Kinematic distributions of the BDT input variables normalised to unity, after the BDTSR event selection. The SM background and the vector-like $B$ quark signal samples corresponding to masses of 1.0~\TeV{}, 1.3~\TeV{}, and 1.5~\TeV{} for \BR($B \to Wt$) =1, respectively. }
\label{fig:BDT1}
\end{figure}

\begin{figure}[h!]
\centering
\includegraphics[width=0.44\textwidth]{figures/bdtIn_sleadjet_pt.pdf}
\includegraphics[width=0.44\textwidth]{figures/bdtIn_MWT.pdf}

\includegraphics[width=0.44\textwidth]{figures/bdtIn_spericityLjets.pdf}
\includegraphics[width=0.44\textwidth]{figures/bdtIn_dR_lepleadjet.pdf}

\includegraphics[width=0.44\textwidth]{figures/bdtIn_dR_WlepleadLjet.pdf}
\includegraphics[width=0.44\textwidth]{figures/bdtIn_dR_lepsleadbjet.pdf}

\includegraphics[width=0.44\textwidth]{figures/bdtIn_MET.pdf}
\includegraphics[width=0.44\textwidth]{figures/bdtIn_hadW_pt.pdf}

\includegraphics[width=0.44\textwidth]{figures/bdtIn_jets_n.pdf}
\includegraphics[width=0.44\textwidth]{figures/bdtIn_hadsleadLjet_pt.pdf}

\caption{ (Continued) Kinematic distributions of the BDT input variables normalised to unity, after the BDTSR event selection. The SM background and the vector-like $B$ quark signal samples corresponding to masses of 1.0~\TeV{}, 1.3~\TeV{}, and 1.5~\TeV{} for \BR($B \to Wt$) =1, respectively.}
\label{fig:BDT2}
\end{figure}

\begin{landscape}
\begin{table}[htbp]
\begin{center}
  \caption{List of the 20 BDT input variables used in the training of the BDTSR, ordered by their TMVA ranking. The terms leading, sub-leading, etc. refer to the \pt\ ordering of the objects.}
\label{tab:BDTvariables}
\begin{tabular}{l|l}
\hline\hline
 Variable & Description \\
\hline \hline
 \ST  &   Scalar sum of \met{}, the \pt\ of the lepton and the \pt\ of all small-$R$ jets\\
  m (leading large-$R$ jet) &   Mass of the leading large-$R$ jet \\
   Sphericity  & Sphericity~\cite{sphericity2} ($\mathcal{S}=\frac{2}{3}(\lambda_{2}+\lambda_{3})$)  is a measure of the total transverse momentum with respect to \\ &  the sphericity axis defined by the four-momenta used for the event shape measurement; $\lambda_{2,3}$ are \\ & the two smallest  eigenvalues of the normalised momentum tensor of the small-$R$ jets, lepton and $\nu$  \\
 $\Delta R(\mathrm{lep}$, sub-leading small-$R$ jet$)$  &   Angular separation between the lepton and the sub-leading small-$R$ jet \\
 $\Delta R($leading $b$-jet, leading large-$R$ jet$)$  &   Angular separation between the leading $b$-tagged jet and the leading large-$R$ jet \\
 min[$\Delta R(\mathrm{lep}$, $b$-jet)]  & Minimum angular separation between the lepton and all $b$-tagged jets \\
 Aplanarity ($\mathcal{A}=\frac{2}{3}\lambda_{3}$)  & Aplanarity~\cite{sphericity2}, where $\lambda_{3}$ is the smallest eigenvalue of the norm. momentum tensor of small-$R$ jets,\\ & lepton and $\nu$ \\
 min[M($W_\text{lep}$, $b$-jet)]  & Minimum invariant mass of $W_\text{lep}$ and all $b$-tagged jets \\
 $\Delta R(\mathrm{lep}$, third-leading small-$R$ jet$)$  &   Angular separation between the lepton and the third-leading small-$R$ jet \\
 $\Delta R(W_\text{lep}$, large-$R$ jet closest to leading $b$-jet$)$  &   Angular separation between the $W_\text{lep}$ and the large-$R$ jet closest to the leading $b$-tagged jet \\
 \pT(sub-leading large-$R$ jet)  &  Transverse momentum of the sub-leading large-$R$ jet \\
 $M^W_T$ &  Transverse mass of the $W_\text{lep}$ \\
 Sphericity (large-$R$ jets)  & Sphericity, using normalised momentum tensor of the large-$R$ jets, lepton and $\nu$ \\
 $\Delta R(\mathrm{lep}$, leading small-$R$ jet$)$  &   Angular separation between the lepton and the leading small-$R$ jet \\
 $\Delta R(W_\text{lep}$, leading large-$R$ jet$)$  &   Angular separation between the $W_\text{lep}$ and the leading large-$R$ jet \\
 $\Delta R(\mathrm{lep}$, sub-leading $b$-jet$)$  &   Angular separation between the lepton and the sub-leading $b$-tagged jet  \\
  \met  &  Missing transverse momentum \\
  \pT($W_\text{had}$)  &  Transverse momenta of the leading $W_\text{had}$ candidate \\
  N$_\text{jets}$ &  Small-$R$ jet multiplicity \\
  \pT(sub-leading small-$R$ jet)  &  Transverse momentum of the sub-leading small-$R$ jet  \\
\hline \hline
\end{tabular}
\end{center}
\end{table}
\end{landscape}

\begin{table}[htbp]
\begin{center}
  \caption{Settings used for the BDT architecture. See Ref.~\cite{TMVA} for further details on these parameters.}
\label{tab:BDTsettings}
\begin{tabular}{l|l}
\hline\hline
 Parameter & Setting \\
 \hline \hline
 Number of trees in the forest & 850 \\
 Maximum depth of the decision tree allowed & 3 \\
 Minimum percentage of training events required in a leaf node & 2.5\% \\
 Number of grid points in variable range used in finding optimal cut in node splitting & 20 \\
 Boosting type for the trees in the forest & AdaBoost \\
 Learning rate for AdaBoost algorithm & 0.5 \\
 Use only a random subsample of all events for growing the trees in each iteration & true \\
 Relative size of bagged event sample to original size of the data sample & 0.5 \\
 Separation criterion for node splitting & GiniIndex \\
  \hline \hline
\end{tabular}
\end{center}
\end{table}

\begin{figure}[h!]
\centering
\includegraphics[width=0.38\textwidth]{figures/VAL_ST.pdf}
\includegraphics[width=0.38\textwidth]{figures/VAL_hadleadLjet_m.pdf}

\includegraphics[width=0.38\textwidth]{figures/VAL_spericity.pdf}
\includegraphics[width=0.38\textwidth]{figures/VAL_dR_lepsleadjet.pdf}

\includegraphics[width=0.38\textwidth]{figures/VAL_dR_leadbjetleadLjet.pdf}

\caption{Pre-fit distributions for the five highest ranked variables used in the BDT training.  From top left these are: $S_T$, m (leading large-$R$ jet), sphericity, $\Delta R(\mathrm{lep}$, sub-leading small-$R$ jet$)$ and $\Delta R($leading $b$-jet, leading large-$R$ jet$)$ . The lower panel shows the ratio of data to the background yields. The band represents the total uncertainty before the maximum-likelihood fit. Events in the overflow and underflow bins are included in the last and first bin of the histograms, respectively. The expected $B\bar{B}$ signal corresponding to $m_{B} = 1300$~\GeV{} for \BR($B \to Wt$) =1 is also shown.}
\label{fig:BDT3}
\end{figure}

\begin{figure}[h!]
\centering
\includegraphics[width=0.38\textwidth]{figures/VAL_ST_postFit.pdf}
\includegraphics[width=0.38\textwidth]{figures/VAL_hadleadLjet_m_postFit.pdf}

\includegraphics[width=0.38\textwidth]{figures/VAL_spericity_postFit.pdf}
\includegraphics[width=0.38\textwidth]{figures/VAL_dR_lepsleadjet_postFit.pdf}

\includegraphics[width=0.38\textwidth]{figures/VAL_dR_leadbjetleadLjet_postFit.pdf}

\caption{Post-fit distributions for the five highest ranked variables used in the BDT training.  From top left these are: $S_T$, m (leading large-$R$ jet), sphericity, $\Delta R(\mathrm{lep}$, sub-leading small-$R$ jet$)$ and $\Delta R($leading $b$-jet, leading large-$R$ jet$)$ . The lower panel shows the ratio of data to the fitted background yields. The band represents the total uncertainty before the maximum-likelihood fit. Events in the overflow and underflow bins are included in the last and first bin of the histograms, respectively. The expected $B\bar{B}$ signal corresponding to $m_{B} = 1300$~\GeV{} for \BR($B \to Wt$) =1 is also shown.}
\label{fig:BDT4}
\end{figure}

\begin{figure}[h!]
\centering
\includegraphics[width=0.98\textwidth]{figures/BDTcorrelations/scat_hadleadLjet_m_vs_ST.pdf}
\caption{Example correlation plot of the two highest ranked BDT input variables: $S_T$ and m (leading large-$R$ jet). The left (right) plot shows the expected correlation for \ttbar\ background ($B\bar{B}$ signal). The signal is shown combining all mass points and for \BR($B \to Wt$) =1, as used in the BDT training.}
\label{fig:BDTcorr}
\end{figure}

\begin{figure}[h!]
\centering
\includegraphics[width=0.8\textwidth]{figures/SR_comp_Wt}
\includegraphics[width=0.8\textwidth]{figures/SR_comp_SU2}
\caption{Comparison of the cross-section limits obtained from the combined fit to the two signal regions, and the fit to each signal region separately. Two signal model cases are shown; a signal model with \BR($B \to Wt$) =1 and a $B$ mass of 1.3~\TeV{} (top) and the SU(2) singlet for a $B$ mass of 1.1~\TeV{} (bottom). For the SU(2) singlet case the BDTSR dominates, while for the \BR($B \to Wt$) = 1 signal model the two signal regions contribute roughly equal. Those masses are chosen as they are close to the expected maximum excluded masses for each scenario. The line at 1 is plotted to guide the eye.}
\label{fig:SRComp}
\end{figure}
